# Supplementary material for: ContraCLM: Contrastive Learning For Causal Language Model
Source: arXiv:2210.01185 source file (2023-05-02)
Supplement: Supplementary file 1 [file text_to_code_stat.tex]

% \begin{table*}[htbp]
%     \begin{center}
%     {\normalsize{
%         % \resizebox{\linewidth}{!} {%
%         \def\arraystretch{1.0}%
%         % \setlength{\tabcolsep}{5pt}
%         \begin{tabular}{l l l l}
%         \toprule
%         & CoSQA  & AdvTest & CSN \\ 
%         \midrule
%         Number of queries               & 500   & 19,210 & 14,918 \\
%         Number of candidate functions   & 6,267 & 19,210 & 43,827  \\
%         Avg. query length               & 7.4   & 13.1   & 12.8 \\
%         Avg. function length            & 79.4  & 175.3  & 170.5 \\
%         \bottomrule
%         \end{tabular}
%         }
%     % }
%     }
%     \caption{
%     Statistics of text-to-code search task datasets.
%     }
%     \label{tab:text_to_code_stat}
%     \end{center}
% \end{table*}
