# Supplementary material for: ContraCLM: Contrastive Learning For Causal Language Model
Source: arXiv:2210.01185 source file (2023-05-02)
Supplement: Supplementary file 2 [file code_search_len_diff.tex]

\begin{table*}[t]
    \begin{center}
    {\normalsize{
        \resizebox{\linewidth}{!} {%
        \def\arraystretch{1.0}%
        % \setlength{\tabcolsep}{5pt}
        \begin{tabular}{l r r r r r r r r r}
        \toprule
        \multirow{2}{*}{Length Diff.} & \multicolumn{3}{c}{\ourmethodtok}  & \multicolumn{3}{c}{\ourmethodseq} & \multicolumn{3}{c}{\ourmethod} \\ 
        \cmidrule(lr){2-4} 
        \cmidrule(lr){5-7}
        \cmidrule(lr){8-10}
        & Ruby & Python & Java & Ruby & Python & Java & Ruby & Python & Java \\ 
        \midrule
        \lbrack 0, 16)      & 23.09 & 27.94 & 17.24 & 21.40 & 22.52 & 16.05 & 22.96 & 26.66 & 17.15 \\
        \hdashline\noalign{\vskip 0.5ex}
        \lbrack 16, 32)      & 17.73 & 20.97 & 12.42 & 16.51 & 16.96 & 10.83 & 17.56 & 20.15 & 12.23 \\
        \hdashline\noalign{\vskip 0.5ex}
        \lbrack 32, 64)      & 17.40 & 17.66 & 12.20 & 16.22 & 14.52 & 10.60 & 17.27 & 17.17 & 12.05 \\
        \hdashline\noalign{\vskip 0.5ex}
        \lbrack 64, 128)    & 14.26 & 13.60 & 9.83 & 13.25 & 11.69 & 8.50 & 14.14 & 13.48 & 9.72 \\
        \hdashline\noalign{\vskip 0.5ex}
        \lbrack 128, 256)   & 8.47 & 8.83 & 5.01 & 7.92 & 7.93 & 4.46 & 8.47 & 8.94 & 4.96 \\
        \hdashline\noalign{\vskip 0.5ex}
        \lbrack 256, 512)   & 2.49 & 3.21 & 0.58 & 2.54 & 2.89 & 0.58 & 2.54 & 3.25 & 0.59 \\
        \bottomrule
        \end{tabular}
        }
    }
    }
    \caption{
    MAP score (\%) of in-language (both query and candidates are in the same language, e.g., Python) code-to-code search task. The ``Length Diff.'' indicates the average length difference (absolute) between queries and their relevant candidate documents. We see a larger performance difference between \ourmethodtok and \ourmethodseq models when length difference is smaller.
    }
    \label{tab:code_to_code_len_diff}
    \end{center}
\end{table*}
